# Supplementary material for: Integrating relative survival in multi-state models -- a non-parametric approach
Source: arXiv:2106.12399 ancillary file (2021-06-23)
Supplement: Supplementary file 1 [file supplementary_material.pdf]

# Supplementary material: Integrating relative survival in multi-state models – a non-parametric approach

Damjan Manevski[1], Hein Putter[2], Maja Pohar Perme[1], Edouard F. Bonneville[2], Johannes Schetelig[3], and Liesbeth C. de Wreede[2]

[1]Institute for Biostatistics and Medical Informatics, Faculty of Medicine, University of Ljubljana, Vrazov trg 2, 1000 Ljubljana, Slovenia
[2]Leiden University Medical Center, Einthovenweg 20 2333 ZC Leiden, the Netherlands
[3]Medical Clinic I, University Hospital, Fetscherstrasse 74, 01307 Dresden, Germany

June 23, 2021

## S1 Population hazard with respect to covariates

$\lambda_P(t)$ is constructed based on demographic covariates. We will write it formally with respect to these covariates. We first denote the population survival curve $S_P(t)$ using $\lambda_P(t)$

$$S_P(t) = \exp(-\int_0^t \lambda_P(u)\,\mathrm{d}u),$$

and write $S_P(t)$ with respect to the covariate distribution

$$S_P(t) = \int S_P(t|\mathbf{x})\,\mathrm{d}H(\mathbf{x}),$$

where $H(\mathbf{x})$ is the covariate distribution function and $S_P(t|\mathbf{x}) = \exp(-\int_0^t \lambda_P(u|\mathbf{x})\,\mathrm{d}u)$ is the expected population survival curve for an individual having covariate values $\mathbf{x}$ (typically a vector of covariates, e.g. age, sex, year at diagnosis), whereas $\lambda_P(t|\mathbf{x})$ is the expected population hazard at time $t$ for an individual having covariate values $\mathbf{x}$.

The population hazard can be then written as

$$\lambda_P(t) = -\frac{d}{dt}\log(S_P(t)),$$

using which we obtain the formula for the hazard

$$\lambda_P(t) = \frac{\int S_P(t|\mathbf{x})\lambda_P(t|\mathbf{x})\,\mathrm{d}H(\mathbf{x})}{S_P(t)}. \tag{1}$$

Note that an equivalent definition of $\lambda_E(t)$ could be given as in (1), but since hazards $\lambda_E(t|\mathbf{x})$ are usually not known (compared to $\lambda_P(t|\mathbf{x})$ which can be obtained from mortality tables) such notation would not be helpful.

An estimator of the cumulative version of the hazard (1) is given in formula (7) in the paper. The integral in formula (1) is replaced by a sum across all individuals in the estimator. The hazards $\lambda_P(t|\mathbf{x})$ are obtained from mortality tables for every individual (depending on demographic covariates $\mathbf{x}$), whereas $S_P(t|\mathbf{x})$ is estimated using the at-risk process $Y(t)$ for every individual. All individuals have an equal weight in the sample, thus $H(\mathbf{x})$ is taken to be uniform across individuals.

# S2 Estimating and evaluating transition hazards and probabilities

An example is provided through which we explain how transition hazards and probabilities are evaluated for split transitions (an illustration of the methods described in Section 2.3). We choose a small dataset to make the different options easier to distinguish.

We generate a dataset of six individuals and fit an extended multi-state model integrating relative survival (using Slovene mortality tables) where the transition diagram is the same as in Figure 3 in the paper. The data for these six individuals is shown in Table S1.

| **Individual** | **Survival time** | **Survival status** | **Relapse time** | **Relapse status** |
|---|---|---|---|---|
| 1 | 10 | 0 | 10 | 0 |
| 2 | 0.33 | 1 | 0.33 | 0 |
| 3 | 0.6 | 1 | 0.6 | 0 |
| 4 | 6.5 | 1 | 6.5 | 0 |
| 5 | 2 | 1 | 1.4 | 1 |
| 6 | 8.4 | 1 | 1 | 1 |

Table S1: The illustrative dataset used in Section S2. The generated times to death an relapse for the six individuals are shown in the table (together with the corresponding event indicators). In case of no observed relapse, the at-risk time for relapse must be equal to the at-risk time for survival.

For this dataset we estimate all transition hazards and probabilities which are shown in Figures S1 and S2. Both split transitions (Alive relapse-free → NRM and Relapse → DaR) have been estimated on daily intervals. On the left side of both figures we show the estimated measures which are evaluated at event times only (and taken to be constant in-between), which is the approach we use by default. On the right side we show the estimates evaluated on a daily basis. We point out that the values on the left and right are equal at event times.

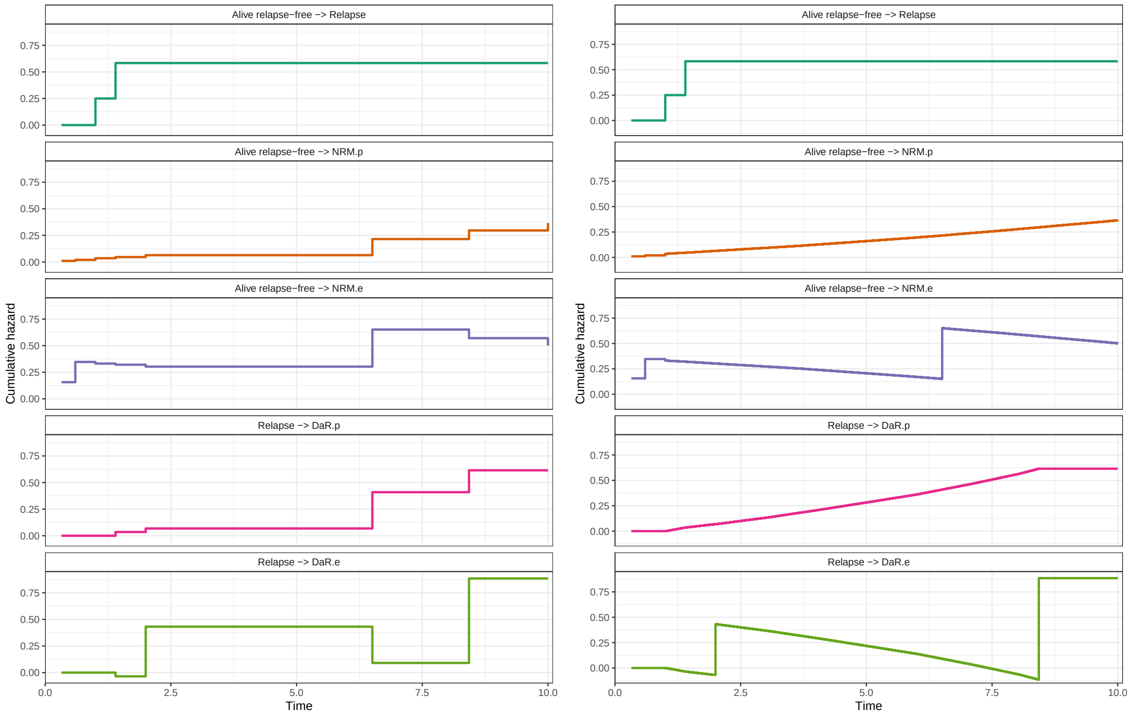


Figure S1: Estimated cumulative hazards for the chosen dataset. On the left side hazard estimates are evaluated at event times only, whereas on the right side they are evaluated on a daily basis. States: Alive relapse-free, Relapse, population NRM (NRM.p), excess NRM (NRM.e), population DaR (DaR.p), excess DaR (DaR.e).

We see that cumulative hazards for population-related transitions are non-decreasing and they increase as long as there is at least one individual in the at-risk set. However, on the left graphs they increase only at event times, whereas on the right the increasing occurs on a daily basis. On the other hand, hazard estimates for excess-related transitions increase whenever an event occurs, and in between event times the estimates decrease (as long as there is someone present in the at-risk set). Although such cumulative hazards might seem unintuitive, in practice they are hardly visible since such decreases are usually small and occur in small intervals. Excess-related hazards can also become negative if there are no events in a longer period. If the measure is negative on large intervals it is wise to reconsider the relative survival assumption (equation (6) in the paper) and whether it is sensible to make the relative survival extension. We note that for non-split transitions the hazard estimates remain the same (Alive relapse-free → Relapse).

In Figure S2 we show the corresponding transition probability estimates. Again, for non-split transitions the estimates are identical. The differences are again visible for the split transitions and they are similar to those of the transition hazards.

For the larger datasets used in practice, the differences between the two approaches become negligible, unless the risk set for a certain transition is small during a part of the follow-up time. As noted, with the default option in our software implementation in `R` we evaluate estimates only at event times, but evaluation at any choice of timepoints is available using argument `add.times` in function

`msfit.relsurv`.

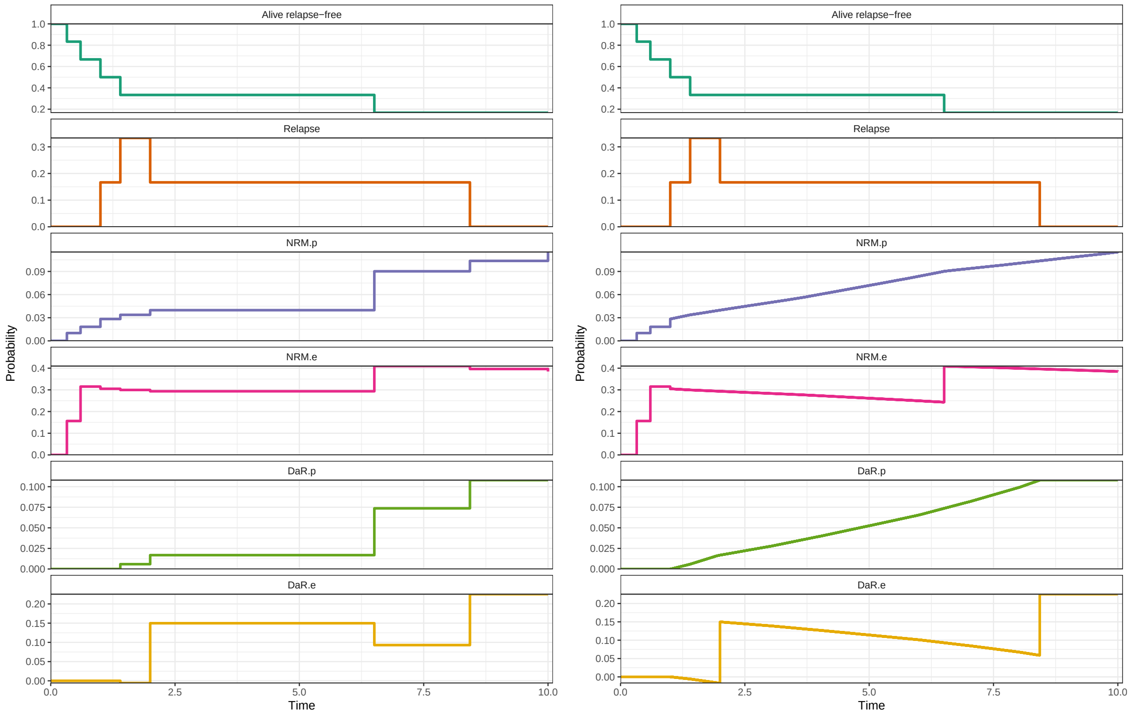


Figure S2: Estimated transition probabilities from starting state Alive relapse-free. On the left side probability estimates are evaluated at event times, whereas on the right side they are evaluated on a daily basis. States: Alive relapse-free, Relapse, population NRM (NRM.p), excess NRM (NRM.e), population DaR (DaR.p), excess DaR (DaR.e).

# S3 Variances for left-truncated hazards

Figure S3 shows the distribution of cumulative hazards for the multi-state model presented in the paper without split death transitions based on 2000 replications with datasets of size 1000. For the two initial transitions (from the starting state to relapse and NRM) the distributions are symmetric and their means increase through time. However, for the transition from relapse to DaR there are some outliers for which the hazard estimates are substantially bigger than most of the values. Such outliers occur when the first event for this transition happens at an early timepoint when only few individuals are already present in state relapse. In such a case, at the first event timepoint for this transition the Nelson-Aalen estimator will make a large jump and consequently the cumulative hazard from then onward is quite bigger than expected.

Consequently, the Greenwood and bootstrap variance estimators for the cumulative hazard underestimate the empirical standard error for left-truncated transitions, which is larger because of these outliers. This is evident in Figure 5 in the paper. We have also checked how the Aalen variance estimator works compared to the two

options (since the Aalen estimator gives an estimate greater than or equal to that of the Greenwood estimator on the hazard level). However, the Aalen estimator does not reach the empirical SE values, thus it is not a suitable alternative.

We note that such a problem has been pointed out in the literature for transition probabilities but not on the hazard level as shown here. At first, the Greenwood estimator was suggested as the most suitable in some earlier work [1], and a similar problem on the probability level has been later exposed [2, 3]. The suggested solutions [2, 3] introduce additional bias when applied to a dataset, thus we do not consider them as completely satisfactory solutions.

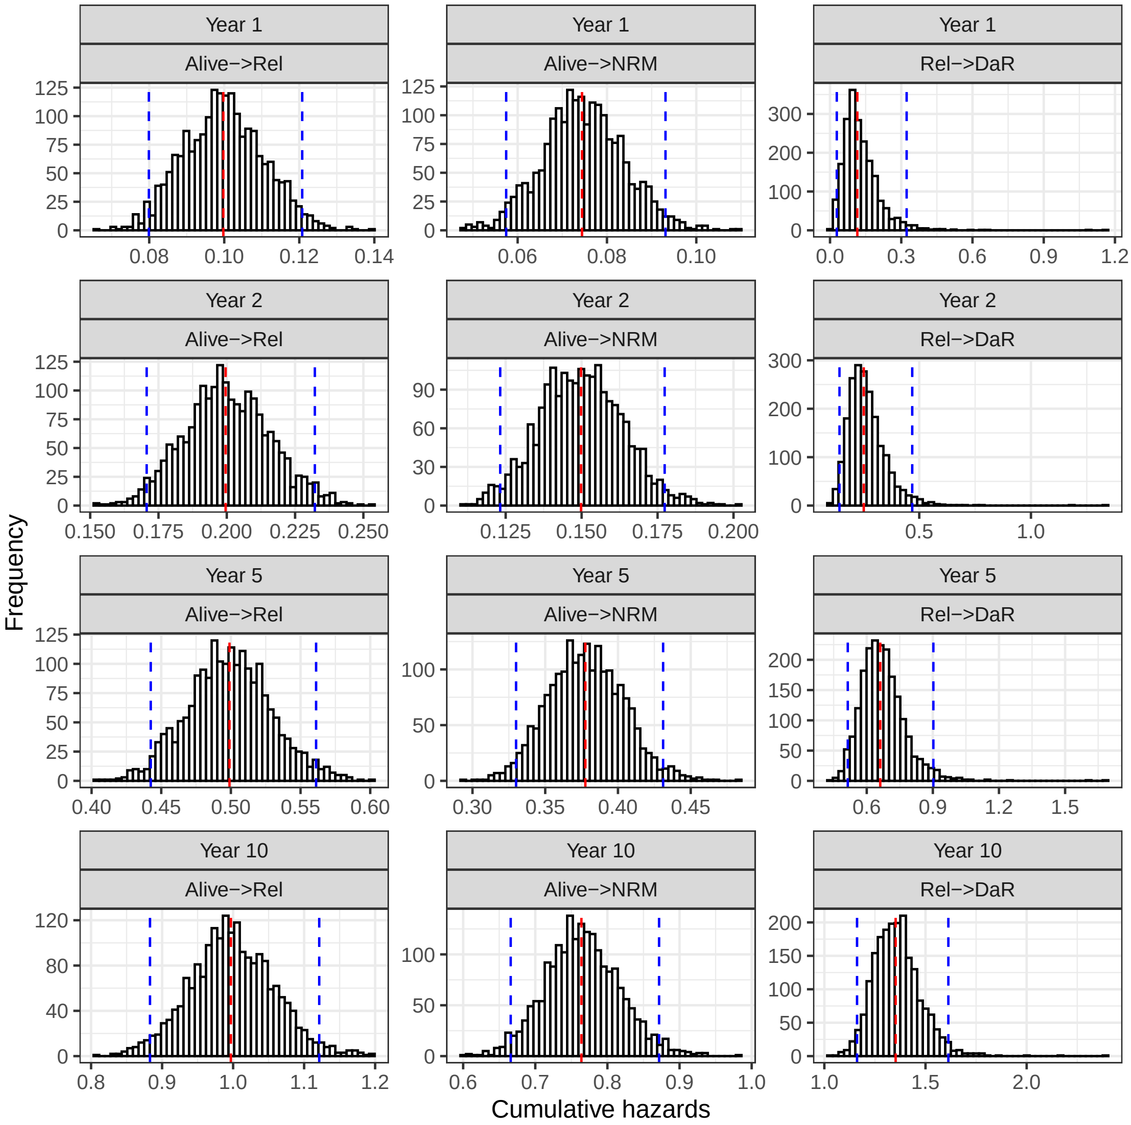


Figure S3: Distribution of cumulative hazards evaluated at times 1, 2, 5 and 10 years for the three transitions in the basic multi-state model, where the death-related transitions are not split in population and excess ones. States: Alive relapse-free (Alive), Relapse (Rel), NRM, DaR. The 2.5% and 97.5% quantiles are shown with blue lines, whereas the median with a red line.

# S4 Example code

The code below shows the full syntax for the analysis presented in Section 4. It presents newly developed functions for this purpose which have been included in the `mstate` package from version 0.3.2 onward (`msfit.relsurv` and an upgrade of `probtrans`) but also rely on functions in the `relsurv` package. The code is available in a separate .R-file (`example_mstaterelsurv.R`), together with a synthetic version of the MDS dataset introduced in Section 4. This dataset contains no identifiable individual patient data but has a very similar structure to the original dataset.

More explanation of the relevant functions in the `mstate` and `relsurv` packages can be found in [? ? ? ], and in the CRAN `mstate` plotting vignette [? ].

```
library(mstate)

# Load synthetic MDS dataset:
load('mds.RData')
head(mds)
#variables:
#id: unique patient identifier
#rfs: relapse-free survival; time to relapse, death or censoring
#(whatever comes first) in years
#srv: overall survival; time to death or censoring
#(whatever comes first) in years
#rel_s: status indicator for relapse (0=censoring, 1=event)
#srv_s: status indicator for death (0=censoring, 1=event)
#age: age at start (alloHCT) in years
#sex: patient sex (male/female)
#dateHCT: date of start (alloHCT), format year-month-day
#country: country of origin of the patient

# Prepare landmark dataset:
# 1. Take patients aged 60 years or older at baseline who are still alive
# relapse-free at 2 years after alloHCT
ids <- mds$id[mds$rfs >= 2 & mds$age>=60]
mds <- mds[mds$id %in% ids,]
# 2. Adjust times and covariates:
mds$rfs <- mds$rfs - 2
mds$srv <- mds$srv - 2
mds$age <- mds$age + 2
mds$dateHCT <- mds$dateHCT + 2*365

# Load mortality tables:
load("joinpoptab.RData")
#this contains the joinpoptab object with all the population mortality
#tables of the countries in the dataset in the format required by the
#functions in the relsurv package (downloaded from www.mortality.org)

# Define the transition matrix:
tmat <- transMat(list(c(2,3),c(4), c(), c()),
    names = c("Alive_relapse-free", "Relapse","NRM", "DaR"))
```

```
# Prepare data in long format using msprep:
mds_msm <- msprep(data=mds, trans=tmat,
    time=c(NA,"rfs", "srv", "srv"),
    status=c(NA, "rel_s", "srv_s", "srv_s"),
    id="id", keep=c("age", "sex", "dateHCT", "country"))

# Coxph object based on msprep object:
cox <- coxph(Surv(Tstart, Tstop, status)~strata(trans),
    data=mds_msm, method="breslow")

# Estimated hazards:
msf <- msfit(cox,trans=tmat, vartype="greenwood")

# Extending the msfit object so that the transitions to death
# are split in excess and population transitions:
msf_relsurv <- msfit.relsurv(msfit.obj = msf, data = mds_msm,
    split.transitions = c(2,3), # which transitions should be split;
    # numbers given in tmat
    ratetable=joinpoptab, # Mortality tables
    # additional mortality tables available: www.mortality.org
    rmap=list(age=age*365.241, year=dateHCT), # link the variable names
    # in the dataset with those in the ratetable;
    # note age has to be given in days
    time.format = "years", # the time unit used in the data
    # options available are 'days', 'years', 'months'
    var.pop.haz = 'bootstrap', # how variance should be estimated
    # other options: 'fixed' (Greenwood) or 'both'
    B=100, # number of bootstrap replications
    # (only relevant if var.pop.haz='bootstrap')
    add.times=5 # additionally evaluate hazards at given timepoints (here
)

# Estimate the transition probabilities:
pt <- probtrans(msf_relsurv, predt=0, direction="forward",
    method="greenwood")

# Estimated cumulative hazards with the corresponding
# bootstrap standard errors at 1,2, 5 years:
summary(msf_relsurv, times = c(1,2,5))
# Estimated transition probabilities together with the corresponding
# bootstrap standard errors and log.boot confidence intervals
# at 1,2, 5 years:
summary(object = pt, times = c(1,2,5), conf.type = 'log')

# Plotting the measures:
plot(msf_relsurv, use.ggplot = TRUE)
plot(pt, use.ggplot = TRUE)
```

# S5 Additional graphs

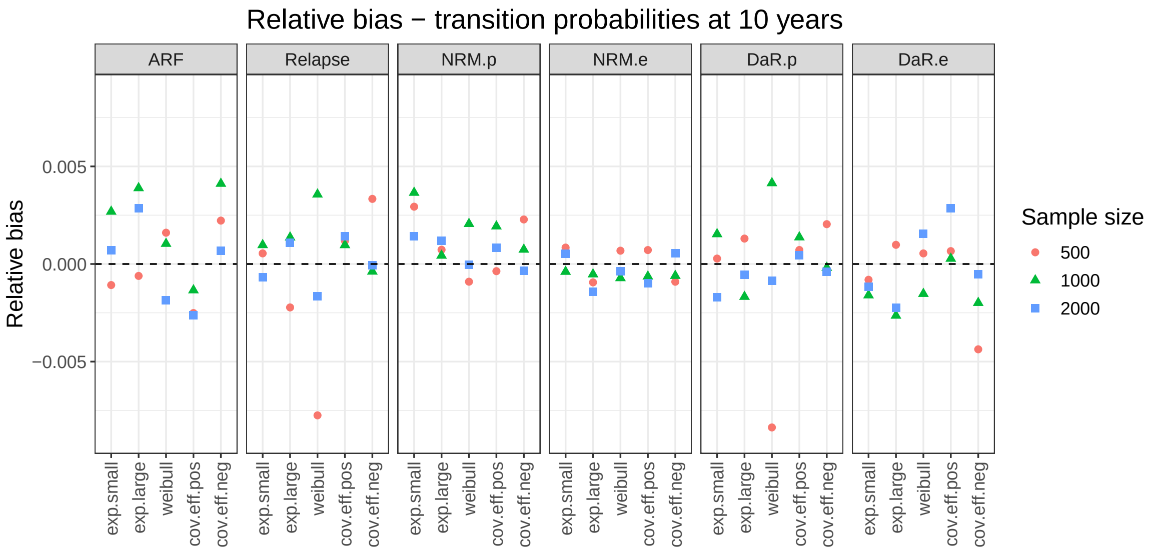


Figure S4: Relative bias for transition probabilities evaluated at end of follow-up (10 years). States: Alive relapse-free (ARF), Relapse, population NRM (NRM.p), excess NRM (NRM.e), population DaR (DaR.p), excess DaR (DaR.e).

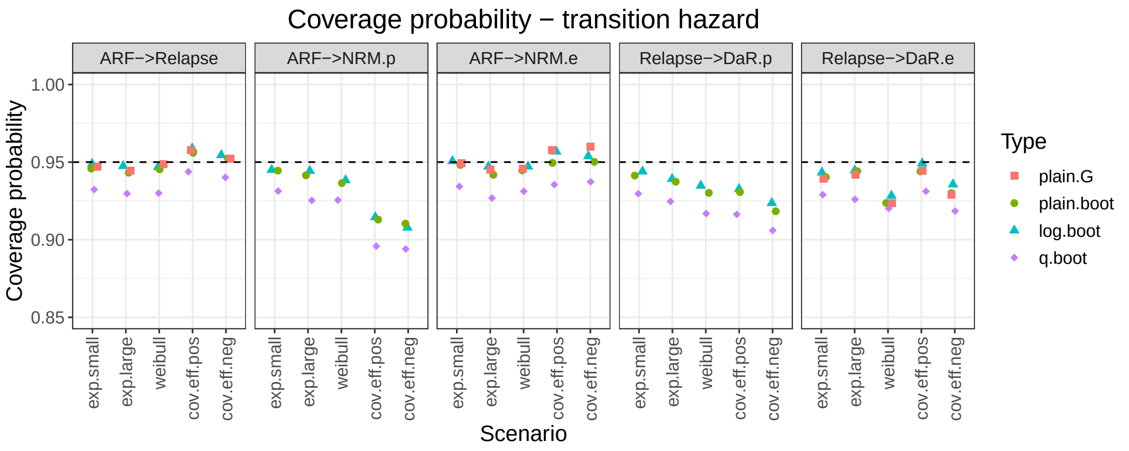


Figure S5: Coverage probabilities for transition hazards evaluated at end of follow-up (10 years) (averaged across sample sizes). Method *plain.G* gives coverage probabilities equal to zero for population NRM and population DaR, thus they are not shown in the figure. States: Alive relapse-free (ARF), Relapse, population NRM (NRM.p), excess NRM (NRM.e), population DaR (DaR.p), excess DaR (DaR.e).

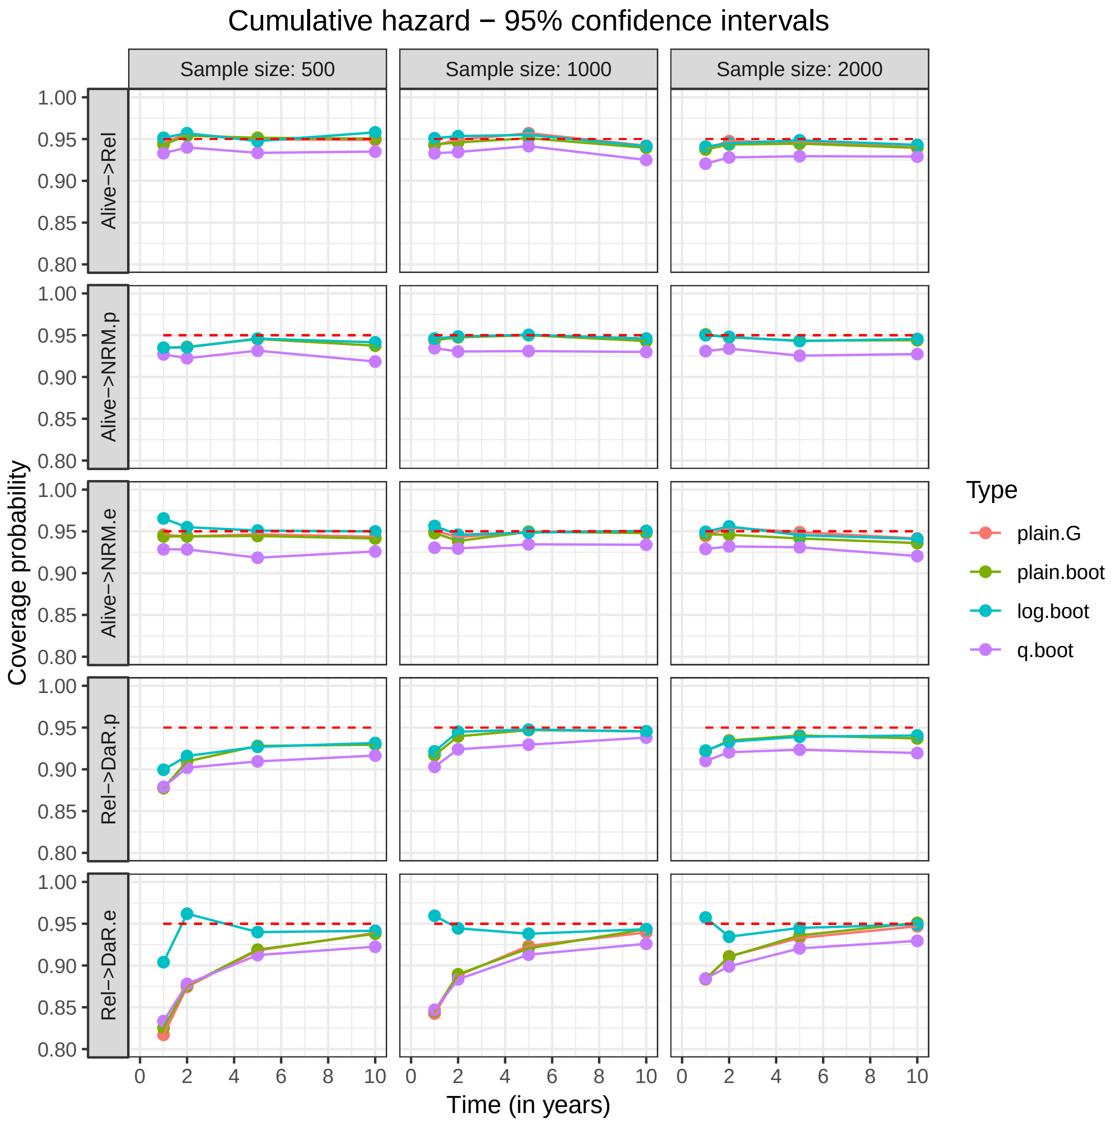


Figure S6: Coverage probabilities for 95% confidence intervals calculated for cumulative hazards - scenario *exp.large*. Evaluated at 1, 2, 5 and 10 years and displayed with respect to transition and sample size in simulation. We note that *plain.G* leads to zero-width confidence intervals for the population transitions, therefore the coverage probability is equal to zero and is not included in the corresponding graphs. States: Alive relapse-free (Alive), Relapse (Rel), population NRM (NRM.p), excess NRM (NRM.e), population DaR (DaR.p), excess DaR (DaR.e).

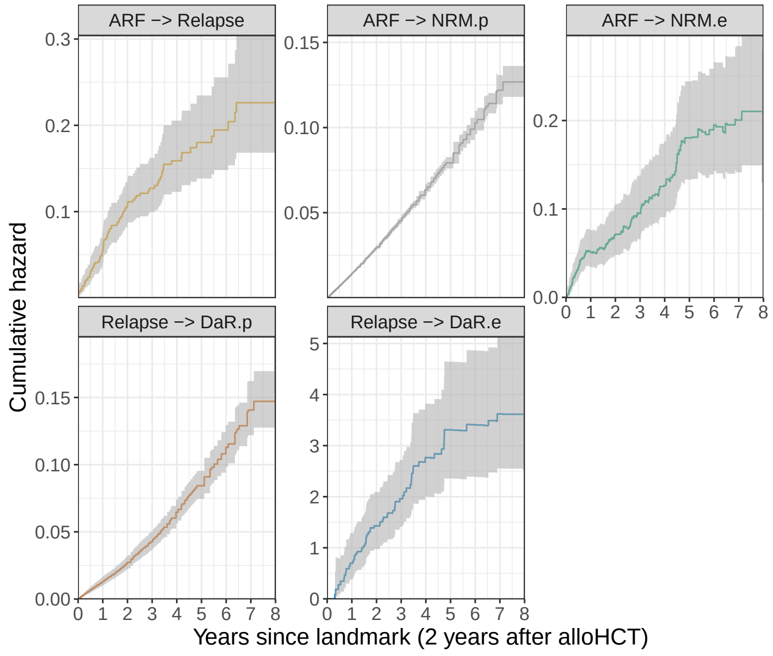


Figure S7: Estimated cumulative hazards with corresponding 95% confidence intervals (method *log.boot*) for the example from Section 4. States: Alive relapse-free (ARF), Relapse (Relapse), population NRM (NRM.p), excess NRM (NRM.e), population DaR (DaR.p), excess DaR (DaR.e).

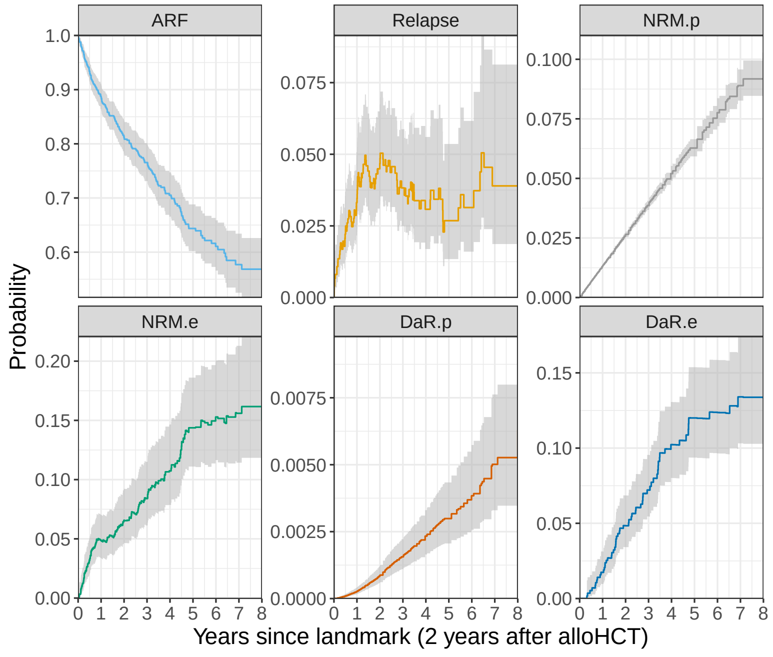


Figure S8: Estimated transition probabilities with the corresponding 95% confidence intervals (method *log.boot*) for the example from Section 4. States: Alive relapse-free (ARF), Relapse (Relapse), population NRM (NRM.p), excess NRM (NRM.e), population DaR (DaR.p), excess DaR (DaR.e).

# S6 Exact parameters and proportions of events for simulation

Let NRM.e denote excess NRM, NRM.p denote population NRM, DaR.e denote excess DaR and DaR.p denote population DaR.

1. ***exp.small***

   Demographic covariates: Sex $\sim$ Bernoulli(0.5), Age $\sim$ Uniform[30, 60], Date of diagnosis $\sim$ Uniform[1990-01-01, 2000-01-01].

   Event times:

   - Alive relapse-free$\rightarrow$NRM.e $\sim$ Exp(0.07),
   - Alive relapse-free$\rightarrow$Relapse $\sim$ Exp(0.10),
   - Relapse$\rightarrow$DaR.e $\sim$ Exp(0.13),
   - Alive relapse-free$\rightarrow$NRM.p and Relapse$\rightarrow$DaR.p are simulated based on population mortality tables,
   - Censoring $\sim$ Exp(0.036).

   Using this setting, at the end of the follow-up (after 10 years), the following distribution holds:

   (a) Including censoring:

   - 12% of the patients remain at state Alive relapse-free, 30% reach NRM.e, 2% reach NRM.p, 41% reach Relapse, the rest of them (15%) were censored before 10 years in the starting state,
   - Out of the 41% that reach Relapse, 20% experience DaR.e, 1% experience DaR.p, 15% reach end of follow-up (i.e. stay in relapse) and 5% are censored.

   (b) Without censoring:

   - 17% of the patients remain at state Alive relapse-free, 33% reach NRM.e, 3% reach NRM.p, 47% reach Relapse,
   - Out of the 47% that reach Relapse, 25% experience DaR.e, 1% experience DaR.p and 20% reach end of follow-up (i.e. stay in relapse).

2. ***exp.large***

   Demographic covariates: Sex $\sim$ Bernoulli(0.5), Age $\sim$ Uniform[55, 85], Date of diagnosis $\sim$ Uniform[1990-01-01, 2000-01-01].

   Event times:

   - Alive relapse-free$\rightarrow$NRM.e $\sim$ Exp(0.055),
   - Alive relapse-free$\rightarrow$Relapse $\sim$ Exp(0.10),
   - Relapse$\rightarrow$DaR.e $\sim$ Exp(0.16),

- Alive relapse-free→NRM.p and Relapse→DaR.p are simulated based on population mortality tables,
- Censoring ~ Exp(0.038).

Using this setting, at the end of the follow-up (after 10 years), the following distribution holds:

(a) Including censoring:

  - 9% of the patients remain at state Alive relapse-free, 20% reach NRM.e, 20% reach NRM.p, 38% reach Relapse, the rest of them (14%) were censored before 10 years in the starting state,
  - Out of the 38% that reach Relapse, 19% experience DaR.e, 7% experience DaR.p, 8% reach end of follow-up (i.e. stay in relapse) and 4% are censored.

(b) Without censoring:

  - 12% of the patients remain at state Alive relapse-free, 23% reach NRM.e, 23% reach NRM.p, 42% reach Relapse,
  - Out of the 42% that reach Relapse, 22% experience DaR.e, 8% experience DaR.p and 11% reach end of follow-up (i.e. stay in relapse).

3. ***weibull***

Demographic covariates: Sex ~ Bernoulli(0.5), Age ~ Uniform[25, 75], Date of diagnosis ~ Uniform[1990-01-01, 2000-01-01].

Event times:

- Alive relapse-free→NRM.e ~ Weibull(a=0.2118, b=0.5278),
- Alive relapse-free→Relapse ~ Weibull(a=0.2044, b=0.5818),
- Relapse→DaR.e ~ Weibull(a=6, b=0.1370),
- Alive relapse-free→NRM.p and Relapse→DaR.p are simulated based on population mortality tables,
- Censoring ~ Exp(0.0525),

where the Weibull distribution is defined with parameters a and b based on the following hazard: $\lambda(t) = abt^{b-1}$.

Using this setting, at the end of the follow-up (after 10 years), the following distribution holds:

(a) Including censoring:

  - 11% of the patients remain at state Alive relapse-free, 33% reach NRM.e, 5% reach NRM.p, 34% reach Relapse, the rest of them (17%) were censored before 10 years in the starting state,

- Out of the 34% that reach Relapse, 25% experience DaR.e, 1% experience DaR.p, 5% reach end of follow-up (i.e. stay in relapse) and 3% are censored.

(b) Without censoring:

- 19% of the patients remain at state Alive relapse-free, 36% reach NRM.e, 6% reach NRM.p, 39% reach Relapse,
- Out of the 39% that reach Relapse, 29% experience DaR.e, 1% experience DaR.p and 9% reach end of follow-up (i.e. stay in relapse).

4. ***cov.eff.pos***

Demographic covariates: Sex $\sim$ Bernoulli(0.5), Age $\sim$ Uniform[55, 85], Date of diagnosis $\sim$ Uniform[1990-01-01, 2000-01-01].

Hazards for the event times:

- Alive relapse-free→NRM.e $= 0.055 \cdot \exp(0.1 \cdot \text{age\_c})$ (age_c is defined as age minus the mean age),
- Alive relapse-free→Relapse $= 0.1 \cdot \exp(0.1 \cdot \text{age\_c})$,
- Relapse→DaR.e $= 0.16$,
- Alive relapse-free→NRM.p and Relapse→DaR.p are simulated based on population mortality tables,
- Censoring $= 0.038$.

Using this setting, at the end of the follow-up (after 10 years), the following distribution holds:

(a) Including censoring:

- 14% of the patients remain at state Alive relapse-free, 20% reach NRM.e, 15% reach NRM.p, 36% reach Relapse, the rest of them (15%) were censored before 10 years in the starting state,
- Out of the 36% that reach Relapse, 17% experience DaR.e, 8% experience DaR.p, 7% reach end of follow-up (i.e. stay in relapse) and 4% are censored.

(b) Without censoring:

- 20% of the patients remain at state Alive relapse-free, 22% reach NRM.e, 17% reach NRM.p, 40% reach Relapse,
- Out of the 40% that reach Relapse, 21% experience DaR.e, 10% experience DaR.p and 9% reach end of follow-up (i.e. stay in relapse),

5. ***cov.eff.neg***

Demographic covariates: Sex $\sim$ Bernoulli(0.5), Age $\sim$ Uniform[55, 85], Date of diagnosis $\sim$ Uniform[1990-01-01, 2000-01-01].

Hazards for the event times:

- Alive relapse-free→NRM.e = $0.055 \cdot \exp(0.1 \cdot \text{age\_c})$ (age_c is defined as age minus the mean age),
- Alive relapse-free→Relapse = $0.1 \cdot \exp(-0.1 \cdot \text{age\_c})$,
- Relapse→DaR.e = 0.16,
- Alive relapse-free→NRM.p and Relapse→DaR.p are simulated based on population mortality tables,
- Censoring = 0.038.

Using this setting, at the end of the follow-up (after 10 years), the following distribution holds:

(a) Including censoring:

- 7% of the patients remain at state Alive relapse-free, 25% reach NRM.e, 19% reach NRM.p, 35% reach Relapse, the rest of them (14%) were censored before 10 years in the starting state,
- Out of the 35% that reach Relapse, 19% experience DaR.e, 4% experience DaR.p, 8% reach end of follow-up (i.e. stay in relapse) and 4% are censored.

(b) Without censoring:

- 11% of the patients remain at state Alive relapse-free, 28% reach NRM.e, 22% reach NRM.p, 39% reach Relapse,
- Out of the 39% that reach Relapse, 22% experience DaR.e, 5% experience DaR.p and 12% reach end of follow-up (i.e. stay in Relapse).

# References


[1] Arthur Allignol, Martin Schumacher, and Jan Beyersmann. A note on variance estimation of the aalen–johansen estimator of the cumulative incidence function in competing risks, with a view towards left-truncated data. *Biometrical Journal*, 52(1):126–137, 2010. doi: 10.1002/bimj.200900039. URL `https://onlinelibrary.wiley.com/doi/abs/10.1002/bimj.200900039`.

[2] Sarah Friedrich, Jan Beyersmann, U. Winterfeld, Martin Schumacher, and Arthur Allignol. Nonparametric estimation of pregnancy outcome probabilities. *The Annals of Applied Statistics*, 11:840–867, 06 2017. doi: 10.1214/17-AOAS1020.

[3] Valentin Rousson, Arthur Allignol, Alexandre Aurousseau, Ursula Winterfeld, and Jan Beyersmann. Stabilizing cumulative incidence estimation of pregnancy outcome with delayed entries. *Biometrical Journal*, 61(5):1290–1302, 2019. doi: 10.1002/bimj.201700237. URL `https://onlinelibrary.wiley.com/doi/abs/10.1002/bimj.201700237`.
